# Supplementary material for: RCCDA: Adaptive Model Updates in the Presence of Concept Drift under a Constrained Resource Budget
Source: arXiv:2505.24149 source file (2026-01-15)
Supplement: Supplementary file 1 [file _Adam___Arxiv____Supplemental_Material_Additional_Results.pdf]

---

# Supplemental Material: Additional Experimental Results

---

## 1 Main Result on OfficeHome Dataset

In this section, we provide additional results on the OfficeHome dataset, a domain generalization dataset which consists of 4 domains: RealWorld, Clipart, Art, and Product. More details on this dataset are available in the “Supplemental Material: Detailed Experimental Setup” document.

The results are shown in Table L1. They are consistent with our results from the other two datasets in Sec. 6 of the main manuscript, with RCCDA achieving significant performance improvements for the Burst and Spikes schedules, moderate improvements for the Wave schedule, and closely matching the best performance for the Step schedule. This further demonstrates the effectiveness of our policy.

Table L1: Average validation accuracy of policies across concept drift schedules for the OfficeHome dataset. The mean update rate constraint is taken as  $\frac{\bar{\lambda}}{\lambda} = 0.1$ . We see that RCCDA consistently outperforms the other methods, with the largest improvement for Burst and Spikes drift schedules.

| Policy<br>Drift Schedule | OfficeHome            |                       |                       |                       |
|--------------------------|-----------------------|-----------------------|-----------------------|-----------------------|
|                          | Burst                 | Step                  | Wave                  | Spikes                |
| <b>RCCDA (ours)</b>      | <b>86.9</b> $\pm$ 2.8 | <b>90.0</b> $\pm$ 1.8 | <b>87.5</b> $\pm$ 2.9 | <b>89.9</b> $\pm$ 2.9 |
| Uniform                  | 81.9 $\pm$ 3.3        | 88.9 $\pm$ 2.5        | 85.0 $\pm$ 3.0        | 85.8 $\pm$ 5.2        |
| Periodic                 | 82.8 $\pm$ 3.5        | <b>89.6</b> $\pm$ 2.2 | 86.3 $\pm$ 3.0        | 88.3 $\pm$ 4.8        |
| Budget-Increase          | 70.7 $\pm$ 4.7        | <b>89.3</b> $\pm$ 2.2 | 85.4 $\pm$ 3.2        | 79.3 $\pm$ 3.7        |
| Budget-Threshold         | 77.7 $\pm$ 5.2        | 85.4 $\pm$ 2.6        | 79.2 $\pm$ 7.5        | 87.7 $\pm$ 2.4        |

## 2 Additional Drift Schedules

In this section, we provide further results on 3 additional drift schedules for the PACS and DigitsDG datasets. The new drift schedules are: (v) *Constant* - the dataset shifts steadily over time, with new domains gradually coming in at a consistent pace, following a predictable pattern. (vi) *Decaying Spikes* - every so often, the dataset gets hit with sudden changes, bringing in new domains with a high drift rate, however these spikes grow less frequent as time goes on. (vii) *Seasonal Flux* - the dataset flows back and forth between two different domains, following a sinusoidal pattern with medium amplitude and long period.

The results are shown in Table L2. They are consistent with our results from drift schedules (i)-(iv), demonstrating once again that RCCDA outperforms the proposed baselines by noticeable margins across all of the new configurations.

## 3 Different Update Rates

Finally, we provide results for different update rate constraint values  $\frac{\bar{\lambda}}{\lambda}$ . The results are given in Figure L1, and offer several new interesting insights. Firstly, our policy closely matches the desired update rate constraint for all values, further validating its adherence to resource constraints. Next,

Table L2: Average validation accuracy of policies across new concept drift schedules for the PACS and DigitsDG datasets. The mean update rate constraint is  $\bar{\lambda}/\lambda = 0.1$ . We see that RCCDA consistently outperforms or matches the baseline algorithms.

| Policy              | PACS                             |                                  |                                  | Digits-DG                        |                                   |                                  |
|---------------------|----------------------------------|----------------------------------|----------------------------------|----------------------------------|-----------------------------------|----------------------------------|
|                     | Constant                         | Decaying Spikes                  | Seasonal Flux                    | Constant                         | Decaying Spikes                   | Seasonal Flux                    |
| <b>RCCDA (ours)</b> | <b>54.1 <math>\pm</math> 1.5</b> | <b>59.7 <math>\pm</math> 3.3</b> | <b>63.4 <math>\pm</math> 2.8</b> | <b>58.1 <math>\pm</math> 9.4</b> | <b>54.5 <math>\pm</math> 15.4</b> | <b>63.7 <math>\pm</math> 9.6</b> |
| Uniform             | 51.3 $\pm$ 1.3                   | 48.0 $\pm$ 5.9                   | 55.1 $\pm$ 6.0                   | 56.2 $\pm$ 7.2                   | 48.0 $\pm$ 12.7                   | 61.9 $\pm$ 8.2                   |
| Periodic            | 48.4 $\pm$ 3.5                   | 51.3 $\pm$ 4.4                   | 57.9 $\pm$ 5.8                   | 56.8 $\pm$ 8.2                   | 49.6 $\pm$ 14.0                   | 62.0 $\pm$ 8.3                   |
| Budget-Increase     | 47.4 $\pm$ 2.4                   | 42.1 $\pm$ 6.1                   | 53.3 $\pm$ 4.3                   | 55.6 $\pm$ 9.3                   | 45.1 $\pm$ 16.8                   | 61.4 $\pm$ 9.9                   |
| Budget-Threshold    | 45.5 $\pm$ 3.7                   | 44.6 $\pm$ 10.9                  | 58.2 $\pm$ 14.5                  | 52.3 $\pm$ 6.7                   | 49.0 $\pm$ 14.8                   | 61.5 $\pm$ 11.5                  |

RCCDA outperforms each of the policies in terms of achieved accuracy for variations in both the real update rate as well as the update rate constraint. The only exception to this is the Budget-Threshold policy on the DigitsDG dataset for values of the real update rate between 0.10 and 0.15. This is most likely the result of different resource availability between the two policies at that point. RCCDA is designed to maximally utilize resources, resulting in the update rate being limited at any time by the constraint. On the other hand, the points in Budget-Threshold policy for update rates 0.10 to 0.15 actually correspond to higher update rate. This allows it to respond faster to change in drift; however, since the actual resource constraint is higher, there is no direct way to control the update rate and ensure it will remain between 0.10 and 0.15. Conversely, when evaluating the accuracy at their desired update rates  $\bar{\lambda}/\lambda$ , we see that our policy outperforms other policies for all rates, demonstrating its effective use of resources and adherence to the constraints.

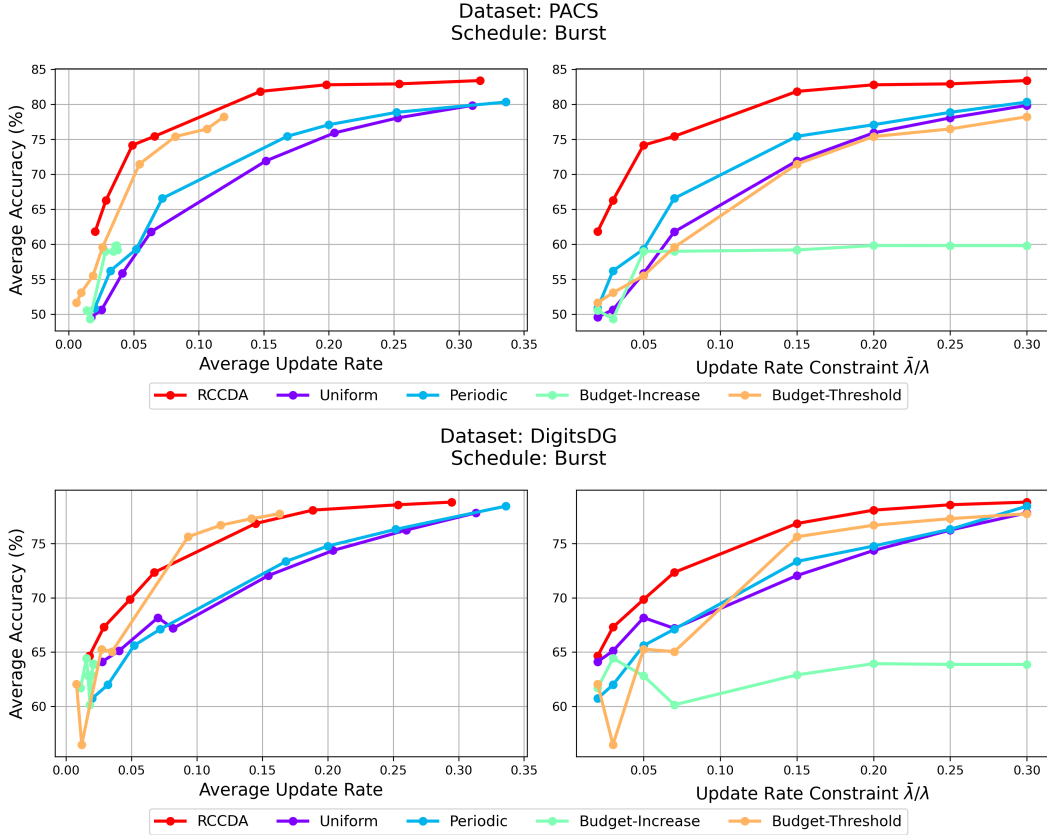

Figure L1: Average validation accuracy of policies across different update rates for the burst drift schedule, across PACS and DigitsDG datasets. The left column is the accuracy per real update rate, and the right column is the accuracy per constrained update rate  $\bar{\lambda}/\lambda$ .
