# Supplementary material for: RCCDA: Adaptive Model Updates in the Presence of Concept Drift under a Constrained Resource Budget
Source: arXiv:2505.24149 source file (2026-01-15)
Supplement: Supplementary file 2 [file _Adam___Arxiv____Supplemental_Material_Documentation.pdf]

---

# Supplemental Material: Detailed Experimental Setup, Documentation

---

## 1 Detailed Experimental Setup

Our experiments are comprised of 2 main phases. First is the *pretraining phase*, which trains the models (described in 1.2) on each of the domains in the datasets (described in 1.1) until convergence. The *evaluation phase* then sees the agent deploy the trained model into an environment that simulates concept drift by introducing new domains, and utilizes a retraining policy to mitigate that drift.

Below we describe each part of the experimental setup in detail. For all datasets, we run the pretraining and evaluation for 3 seeds and average the results.

### 1.1 Datasets

To simulate concept drift in our experiments, we utilized 3 common domain generalization (DG) datasets:

- **PACS** [1]: PACS consists of images from 4 domains: Photo, Art Painting, Cartoon, and Sketch, each with the 7 common categories: dog, elephant, giraffe, guitar, horse, house, and person. The default size of the images is  $224 \times 224$ . We transform all images into  $128 \times 128$ .
- **DigitsDG** [2]: DigitsDG encompasses images of handwritten digits 0 to 9, sourced from 4 different domains: SVHN, SYN, MNIST, and MNIST-M, corresponding to 4 original distinct datasets. The image sizes are  $32 \times 32$ .
- **OfficeHome** [3]: OfficeHome consists of images from four domains: Art, Clipart, Product, and Real-World, each featuring 65 object categories commonly encountered in office and home environments, including chairs, desks, and household items. The image sizes are  $224 \times 224$ .

### 1.2 Models

Below, we specify the models employed for each dataset:

**PACS**. For the PACS dataset, we utilize a custom convolutional neural network (CNN) with skip connections, called PACSCNN. The network architecture, from input to output, is as follows:

| Layer | Layer Description                                                                             |
|-------|-----------------------------------------------------------------------------------------------|
| 1     | Convolutional layer: 3 input channels, 64 output channels, kernel size 3, stride 1, padding 1 |
| 2     | Batch normalization layer                                                                     |
| 3     | ReLU activation                                                                               |
| 4     | Residual block: 64 input channels, 64 output channels, stride 1                               |
| 5     | Residual block: 64 input channels, 64 output channels, stride 1                               |
| 6     | Residual block: 64 input channels, 128 output channels, stride 2                              |
| 7     | Residual block: 128 input channels, 128 output channels, stride 1                             |
| 8     | Residual block: 128 input channels, 256 output channels, stride 2                             |
| 9     | Residual block: 256 input channels, 256 output channels, stride 1                             |
| 10    | Residual block: 256 input channels, 512 output channels, stride 2                             |
| 11    | Residual block: 512 input channels, 512 output channels, stride 1                             |
| 12    | Adaptive average pooling layer: reduces spatial dimensions to $1 \times 1$                    |
| 13    | Flatten operation                                                                             |
| 14    | Dropout layer: $p = 0.5$                                                                      |
| 15    | Linear layer: 512 input features to 7 output classes                                          |

Each residual block has the following structure:

| Layer | Layer Description                                                                                                                       |
|-------|-----------------------------------------------------------------------------------------------------------------------------------------|
| 1     | Convolutional layer: input, output channels, stride, passed as arguments, kernel size 3, padding 1                                      |
| 2     | Batch normalization layer                                                                                                               |
| 3     | ReLU activation                                                                                                                         |
| 4     | Batch normalization layer                                                                                                               |
| 5     | Skip connection, identity when number of input channels equals output channels, otherwise convolutional mapping and batch normalization |
| 6     | ReLU activation                                                                                                                         |

**DigitsDG.** For the DigitsDG dataset, the DigitsDGCNN used has the following layer configuration:

| Layer | Layer Description                                                                                |
|-------|--------------------------------------------------------------------------------------------------|
| 1     | Convolutional layer: 3 input channels, 64 output channels, kernel size 3, stride 1, padding 1    |
| 2     | Batch normalization layer                                                                        |
| 3     | ReLU activation                                                                                  |
| 4     | Convolutional layer: 64 input channels, 64 output channels, kernel size 1, stride 2, padding 0   |
| 5     | Convolutional layer: 64 input channels, 128 output channels, kernel size 3, stride 1, padding 1  |
| 6     | Batch normalization layer                                                                        |
| 7     | ReLU activation                                                                                  |
| 8     | Convolutional layer: 128 input channels, 128 output channels, kernel size 1, stride 2, padding 0 |
| 9     | Convolutional layer: 128 input channels, 256 output channels, kernel size 3, stride 1, padding 1 |
| 10    | Batch normalization layer                                                                        |
| 11    | ReLU activation                                                                                  |
| 12    | Convolutional layer: 256 input channels, 256 output channels, kernel size 1, stride 2, padding 0 |
| 13    | Convolutional layer: 256 input channels, 512 output channels, kernel size 3, stride 1, padding 1 |
| 14    | Batch normalization layer                                                                        |
| 15    | ReLU activation                                                                                  |
| 16    | Convolutional layer: 512 input channels, 512 output channels, kernel size 1, stride 2, padding 0 |
| 17    | Adaptive average pooling layer: reduces spatial dimensions to $1 \times 1$                       |
| 18    | Flatten operation                                                                                |
| 19    | Dropout layer: $p = 0.5$                                                                         |
| 20    | Linear layer: 512 input features to 10 output classes                                            |

**OfficeHome** The network for the OfficeHome dataset, named OfficeHomeNet, is based on the ResNet-18 [4] architecture, adapted for our setting. The original fully connected layer of ResNet-18 is replaced with a new custom one comprised of:

| Layer | Layer Description                                       |
|-------|---------------------------------------------------------|
| 1     | Linear layer: 512 input features to 256 output features |
| 2     | ReLU activation                                         |
| 3     | Dropout layer: $p = 0.5$                                |
| 4     | Batch normalization layer                               |
| 5     | Linear layer: 256 input features to 10 output classes   |

This network also utilizes the pre-trained model parameter weights, with the weights of the initial convolutional layer (conv1), batch normalization layer (bn1), and the first three residual layers (layer1, layer2, layer3) of the Resnet-18 remaining constant throughout the entire experiment.

### 1.3 Pretraining Phase

The pretraining phase initiates with the acquisition of the complete dataset, which is subsequently partitioned into training and holdout sets utilizing an 80:20 split through random uniform sampling. The training set, denoted as  $\mathcal{D}$ , retains a fixed size throughout the training. Following the application of dataset-specific transformations, both the training and holdout datasets are refined to exclusively comprise samples from a single designated source domain. Subsequently, two agents are instantiated: the training agent, tasked with updating the model parameters using the training dataset, and the holdout agent, responsible for assessing the performance of the updated model on the holdout dataset.

Upon initialization of the loss criterion and optimizer, the training loop commences. Within each iteration, the training agent employs the ‘update steps’ method to refine the model parameters. Unlike traditional epoch-based training, this method samples batches, each of size  $|\xi|$ , from the training dataset for  $n_{\text{steps}}$  steps, computing gradients and updating the model with the specified optimizer and learning rate  $\eta$ . This design proves advantageous during the evaluation phase by enabling explicit

control of simulation conditions. Furthermore, increasing the number of steps per update in the pretraining phase allows for faster model optimization, simulating increased computational resources.

After each parameter update, the holdout agent evaluates the revised model on the holdout dataset, calculating evaluation metrics. An early stopping mechanism is also implemented, terminating the training loop if the holdout accuracy exceeds a predefined threshold,  $\text{acc}_{\text{thresh}}$ . At completion of the training loop, both the results and final model parameters are archived for subsequent analysis.

The exact values of hyperparameters and other settings are specific to each dataset and summarized in Table M1, and were chosen experimentally utilizing linear and grid search approaches.

Table M1: Hyperparameter settings for the pretraining phase across PACS, DigitsDG, and OfficeHome datasets.

| Hyperparameter                           | PACS                  | DigitsDG              | OfficeHome                                                  |
|------------------------------------------|-----------------------|-----------------------|-------------------------------------------------------------|
| Learning Rate ( $\eta$ )                 | 0.005                 | 0.05                  | 0.05                                                        |
| Batch Size ( $ \xi $ )                   | 128                   | 128                   | 256                                                         |
| # of Steps/Update ( $n_{\text{steps}}$ ) | 10                    | 10                    | 20                                                          |
| Number of Updates ( $T$ )                | 200                   | 200                   | 100                                                         |
| Loss                                     | Cross Entropy         | Cross Entropy         | Cross Entropy                                               |
| Optimizer                                | SGD                   | SGD                   | SGD                                                         |
| Momentum                                 | 0.9                   | 0.9                   | 0.9                                                         |
| $\text{acc}_{\text{thresh}}$             | 75%                   | 75%                   | 90%                                                         |
| Transforms                               | resize, normalize     | resize, normalize     | random resize crop,<br>random horizontal flip,<br>normalize |
| Normalization Mean                       | [0.485, 0.456, 0.406] | [0.485, 0.456, 0.406] | [0.485, 0.456, 0.406]                                       |
| Normalization Variance                   | [0.229, 0.224, 0.225] | [0.229, 0.224, 0.225] | [0.229, 0.224, 0.225]                                       |

## 1.4 Evaluation Phase

**Dataset and General Setup.** The evaluation phase begins with the full dataset, as described in Section 1.1, partitioned into training and holdout sets using an 80:20 split via random uniform sampling, similar to the pretraining phase. Unlike in the pretraining phase, however, once both datasets are modified to only contain a single source domain, their size is limited to  $|\mathcal{D}_{\text{set}}| \leq |\mathcal{D}|$  and  $0.25 \times |\mathcal{D}_{\text{set}}|$  respectively.

Next, we once again initialize the training and holdout agents, define the loss criterion and optimizer, initialize the loss array tracking all historical loss values, and deploy the agents for  $T = 250$  time slots into an environment experiencing different types of drift. The agent follows a policy to decide when to update given the constraints. We consider a constraint  $\bar{\lambda}$  and a constant update cost  $\lambda$ , and evaluate the setting for different values of the fraction  $\frac{\bar{\lambda}}{\lambda}$ . When the update occurs, it utilizes the ‘update steps’ method with  $n_{\text{steps}}$  steps, batch size of  $|\xi|$ , and learning rate  $\eta$ , similar to the pretraining phase.

The evaluation process update hyperparameters are summarized in Table M2.

**Drift Schedules.** To simulate concept drift, we utilize a drift scheduler that dynamically determines the appropriate drift rates and patterns for any given time  $t$  for different drift types. The new samples are introduced into the training and holdout datasets, replacing the current data not from the target domains. The drift scheduler not only controls the timing, rate, and target domains of a drift type, but also implements a variety of drift schedules, each defining a distinct pattern of new domain introduction.

We implement 7 schedules, with 4 in the main paper, and 3 additional schedules available in the supplemental material. Each schedule uses the ‘replace’ strategy, substituting existing samples with those from the target domains at the specified drift rate (as fraction of the dataset), ensuring dataset size consistency.

Table M2: Update hyperparameter settings for the evaluation phase across PACS, DigitsDG, and OfficeHome datasets.

| Hyperparameter                           | PACS                  | DigitsDG              | OfficeHome            |
|------------------------------------------|-----------------------|-----------------------|-----------------------|
| Learning Rate ( $\eta$ )                 | 0.01                  | 0.05                  | 0.05                  |
| Batch Size ( $ \xi $ )                   | 128                   | 128                   | 256                   |
| # of Steps/Update ( $n_{\text{steps}}$ ) | 5                     | 1                     | 5                     |
| Loss                                     | Cross Entropy         | Cross Entropy         | Cross Entropy         |
| Optimizer                                | SGD                   | SGD                   | SGD                   |
| Transforms                               | resize, normalize     | resize, normalize     | resize, normalize     |
| Normalization Mean                       | [0.485, 0.456, 0.406] | [0.485, 0.456, 0.406] | [0.485, 0.456, 0.406] |
| Normalization Variance                   | [0.229, 0.224, 0.225] | [0.229, 0.224, 0.225] | [0.229, 0.224, 0.225] |

Below we detail the configurations for the PACS dataset; the configurations for DigitsDG and OfficeHome datasets are almost the same, except they have corresponding domains replaced in accordance with their custom dataset domains.

- **Burst:** This introduces new domains in periodic deterministic bursts. Each burst effectively replaces all samples from the current domain with samples from the new domain. After initial delay of 45 time steps with no drift, burst occur at times 45, 165, introducing data from photo and cartoon domains respectively, at rates 0.4 for 3 time steps, effectively replacing the entire dataset.
- **Step:** At times 60, 120, 180, in order, domains Sketch, Cartoon, Art Painting are introduced into the dataset at constant drift rates 0.004, 0.006, 0.008 in-between introduction times respectively.
- **Wave:** After an initial delay of 50, domains are introduced at a rate 0.032 for 30 time steps, followed by 70 time steps of no drift. Domains cycle in the Photo, Cartoon, Sketch order.
- **Spikes:** This extends the Burst schedule with randomized characteristics like the interval between the spikes, spike duration, or initial delay, creating a spiking schedule. The possible spike interval value is between 90 and 130, the initial delay between 30 and 60, the spike duration is between 3 and 6 times slots, and the spike rate between 0.3 and 0.6. The domains cycle in the Photo, Cartoon, Sketch order for the corresponding spikes.
- **Constant:** Here, the drift has a constant rate 0.016, domains cycle every time 50 steps according to: Sketch, Photo, Cartoon, Art Painting schedule.
- **Decaying Spikes:** This is a modification of the Burst schedule, with increasing intervals between the spikes. After an initial delay of 20 a spike happens, and the following spikes occur at increasing intervals. The spike interval starts at 30, and increases by 10 after each spike. Each spike takes 3 time steps, and has a drift rate of 0.35. The domains cycle Sketch, Photo, Cartoon in order for each spike.
- **Seasonal Flux:** This simulates cyclic drift with alternating domains. After an initial delay of 10 time steps, the schedule cycles between the photo and sketch domains, with a full cycle from photo to sketch and back to photo taking 150 time steps. The rate of the drift between 0.001 and 0.016 according to a sine wave.

**Update Policies** The proposed update policy and baselines are implemented (each policy has a corresponding number assigned) as follows:

- **Uniform** (Policy 1): Retrains randomly with probability  $\frac{\lambda}{\bar{\lambda}} = \bar{\pi}$ .
- **Periodic** (Policy 2): Retrains at fixed intervals  $\frac{\lambda}{\bar{\lambda}} = \frac{1}{\bar{\pi}}$
- **Budget-Increase** (Policy 3): Retrains when the loss increases consecutively over a window of size  $w = 40$  for 3 times in a row, if sufficient tokens (budget) are available. Tokens accumulate at rate  $\frac{\lambda}{\bar{\lambda}} = \bar{\pi}$ .
- **Budget-Threshold** (Policy 4): Retrains when the current loss exceeds the maximum loss over a window of size  $w = 40$  by a threshold  $\epsilon = 0.1$ , if sufficient tokens (budget) are available.
- **RCCDA** (Policy 5): The proposed policy with estimation defined as  $\eta LV \left\| \nabla \hat{f}_t \right\| \approx \eta LV \hat{g}(\mathcal{H}_f) = VK_d(f_t - f_{t-1})$ . The update occurs if:  $V \left[ K_p(f_t - \min_{i \in \mathcal{H}_f} f_i) + K_d(f_t - f_{t-1}) \right] \geq Q(t) +$

$0.5 - \frac{\bar{\lambda}}{\lambda}$ . We keep the value of  $V = 10$  constant across all experiments, and adjust  $K_p, K_d$  values for different settings and resource constraints. The virtual queue is updated as  $Q(t+1) = \max \left\{ 0, Q(t) + \pi(t) - \frac{\bar{\lambda}}{\lambda} \right\}$ .

In Tables M3, and M4 we summarize the values of  $K_p, K_d$  used by RCCDA across all conducted experiments.

Table M3:  $(K_p, K_d)$  parameters used by RCCDA for different drift schedules, across PACS, DigitsDG, and OfficeHome

| Drift Schedule  | PACS        | DigitsDG    | OfficeHome |
|-----------------|-------------|-------------|------------|
| Burst           | (1.0, 0.1)  | (2.5, 0.5)  | (1.0, 0.5) |
| Step            | (1.0, 0.1)  | (1.0, 0.5)  | (1.0, 0.5) |
| Wave            | (0.5, 0.1)  | (1.0, 0.5)  | (1.0, 0.5) |
| Spikes          | (0.75, 0.5) | (2.0, 0.1)  | (1.0, 0.5) |
| Constant        | (0.2, 0.1)  | (0.3, 0.25) | N/A        |
| Decaying Spikes | (0.5, 0.1)  | (0.5, 0.1)  | N/A        |
| Seasonal Flux   | (0.3, 0.25) | (0.5, 0.1)  | N/A        |

Table M4:  $(K_p, K_d)$  parameters used by RCCDA for different update rates for the Burst and Step drift schedules, across PACS and DigitsDG

| Update Rate $\frac{\bar{\lambda}}{\lambda}$ | PACS         | DigitsDG     |
|---------------------------------------------|--------------|--------------|
| 0.02                                        | (0.06, 0.05) | (0.1, 0.05)  |
| 0.03                                        | (0.13, 0.05) | (0.28, 0.05) |
| 0.05                                        | (0.5, 0.1)   | (0.55, 0.1)  |
| 0.07                                        | (0.7, 0.1)   | (1.0, 0.2)   |
| 0.15                                        | (4.0, 1.0)   | (4.0, 1.0)   |
| 0.20                                        | (7.0, 2.5)   | (7.0, 2.0)   |
| 0.25                                        | (10.0, 4.0)  | (14.0, 6.0)  |
| 0.30                                        | (14.0, 5.5)  | (20.0, 8.0)  |

**Evaluation Loop** Given such setup, we execute the evaluation loop for  $T = 250$  time steps to simulate operation of an agent in an environment experiencing concept drift over time. At each time  $t$ , the loop executes the following operations:

1. **Apply Drift:** The drift scheduler provides the current drift rate and target domains for the concept drift applied by both agents to their datasets.
2. **Evaluate Performance:** The holdout agent computes the current loss and accuracy on the holdout set, simulating inference task.
3. **Policy Decision:** The selected policy determines whether to retrain based on current and historical metrics.
4. **Retrain if Decided:** If retraining is triggered, the training agent performs  $n_{\text{steps}}$  updates using the optimizer with learning rate  $\eta$ . The holdout agent’s model parameters are updated to the new training agent parameters.

**Results** The results from the main paper are averaged over 10 seeds, while the results in the supplemental material are averaged over 3 seeds. For Figure 2 in the main text, we consider a single starting domain for each of the drift schedules for the PACS dataset. For the numerical results in Table 2 of the main text, we average the results for PACS over starting domains: Photo, Art Painting, Cartoon, Sketch; for DigitsDG over starting domains: mnist, mnist-m, and svhn; and for OfficeHome over starting domains: RealWorld, Product, Art. The reported accuracy for each case is the achieved accuracy on the holdout dataset averaged the entire operation time  $T$ .

## 2 Documentation

In this section, we provide specific details on the code and hardware used for our experiments.

**Code Description** We wrote our code in Python, and used the following imported modules: PyTorch, torchvision, numpy, flwr\_datasets [5], PIL. We implemented a custom package for making the code operation easier. The package code is available under `Federated_Learning_Base_Toolkit_torch`, and includes source code for our core classes and methods, such as `BaseNeuralNetwork` with the ‘update steps’ method, `DriftAgent`, class `DomainDrift`, or the custom datahandlers and datasets. The code in `concept_drift_optimal_adaptation` uses these methods to implement pre-training, drift scheduling, update policies, and the policy evaluation code. We included the source code in the supplemental materials. Further details are available in our implementation.

**Executing Code** The code can be run through the following steps:

1. Navigate to the directory with the code and run the commands:

```
conda install -f cog_fl_llm_env.yml  
conda activate cog_fl_llm_env.yml
```

2. Navigate to directory `Federated_Learning_Base_Toolkit_torch`, and run the package installation command:

```
python -m pip install .
```

3. To pretrain a model navigate to a dataset-specific directory, and run:

```
python3 pretrain_models_dset --options
```

where `dset` is the name of the corresponding dataset, and options specify various parameters of the pretraining, the details are available in the code.

- For DigitsDG and OfficeHome datasets, a root directory with the downloaded dataset has to be specified. In order to run the code for these dataset, one has to download the corresponding dataset, and update the root directory variable to store the path to the download.

4. To evaluate a model, navigate to a dataset-specific directory, and run

```
python3 evaluate_policy_dset --options
```

where options specify various parameters of the evaluation process, the policy evaluated, the setting used, and the drift schedule.

- Similarly to pretraining, for DigitsDG and OfficeHome datasets, a root directory with the downloaded dataset has to be specified in order for the code to work.

**Hardware.** For each experiment, we utilized 14 Intel Xeon Platinum 8480+ CPU cores and 1 NVIDIA H100 GPU. CPU memory was allocated proportionally to the core request, with approximately 9 GB per core, yielding about 126 GB of CPU memory per job. The H100 GPU provided 80 GB of dedicated memory. The GPU executed all seeds concurrently for a given experimental configuration. The upper time limit for pretraining was set to 2 days, and for each evaluation job was set to 6 hours. In practice, the pretraining took at most 2 hours per configuration. More importantly, the evaluation execution time varied by datasets, with the DigitsDG dataset taking 5 minutes per configuration on average, PACS evaluations averaging 15 minutes (up to 20 minutes), and OfficeHome evaluations averaging around 30 minutes per configuration.

## References

- [1] Da Li, Yongxin Yang, Yi-Zhe Song, and Timothy M. Hospedales. Deeper, broader and artier domain generalization, 2017. URL <https://arxiv.org/abs/1710.03077>.
- [2] Kaiyang Zhou, Yongxin Yang, Timothy Hospedales, and Tao Xiang. Learning to generate novel domains for domain generalization. In Andrea Vedaldi, Horst Bischof, Thomas Brox, and Jan-Michael Frahm, editors, *Computer Vision – ECCV 2020*, pages 561–578, Cham, 2020. Springer International Publishing. ISBN 978-3-030-58517-4.
- [3] Hemanth Venkateswara, Jose Eusebio, Shayok Chakraborty, and Sethuraman Panchanathan. Deep hashing network for unsupervised domain adaptation. In *Proceedings of the IEEE Conference on Computer Vision and Pattern Recognition*, pages 5018–5027, 2017.
- [4] Kaiming He, Xiangyu Zhang, Shaoqing Ren, and Jian Sun. Deep residual learning for image recognition, 2015. URL <https://arxiv.org/abs/1512.03385>.
- [5] Daniel J. Beutel, Taner Topal, Akhil Mathur, Xinchu Qiu, Titouan Parcollet, and Nicholas D. Lane. Flower: A friendly federated learning research framework. *CoRR*, abs/2007.14390, 2020. URL <https://arxiv.org/abs/2007.14390>.
